# Supplementary material for: Beyond Models! Explainable Data Valuation and Metric Adaption for Recommendation
Source: arXiv:2502.08685 source file (2025-02-12)
Supplement: Supplementary file 1 [file 8_Appendix.tex]

\newpage
\appendix
\section{Appendix}
\subsection{Metric Optimization}  \label{app:pg}
We utilize the REINFORCE algorithm to optimize the performance metric. The detailed optimization process is proved in the following equations:
    \begin{equation}
        \small
        \begin{aligned}
            &\nabla_{\Lambda}\hat{l}(\Lambda)
            =\nabla_{\Lambda} \mathbb{E}_{s\sim \pi{(\mathcal{B},\cdot;{\Lambda})}} \mathcal{R}(\hat{\mathcal{D}}, f(\Theta^*(\Lambda)))\\
            &=\nabla_{\Lambda}\sum_{s\in[0,1]^{|\mathcal{B}|}} \mathcal{R}(\hat{\mathcal{D}}, f(\Theta^*(\Lambda))) \cdot \pi(\mathcal{B},s;{\Lambda}) \\
            &=\sum_{s\in[0,1]^{|\mathcal{B}|}} \mathcal{R}(\hat{\mathcal{D}}, f(\Theta^*(\Lambda))) \cdot 
            \frac{\nabla_{\Lambda}\pi(\mathcal{B},s;{\Lambda})}{\pi(\mathcal{B},s;{\Lambda})}\cdot \pi(\mathcal{B},s;{\Lambda})\\
            &= \sum_{s\in[0,1]^{|\mathcal{B}|}} \mathcal{R}(\hat{\mathcal{D}}, f(\Theta^*(\Lambda))) \cdot \nabla_{\Lambda}log(\pi(\mathcal{B},s;{\Lambda}))\cdot \pi(\mathcal{B},s;{\Lambda})\\
            &=\mathbb{E}_{s\sim \pi(\mathcal{B},\cdot;{\Lambda})}[\mathcal{R}(\hat{\mathcal{D}}, f(\Theta^*(\Lambda)))\cdot \nabla_{\Lambda}log(\pi(\mathcal{B},s;{\Lambda}))],
        \end{aligned}
    \end{equation}

\subsection{Learning Algorithm}  \label{app:learning_algorithm}
The detailed optimization steps of the proposed framework are given in Algorithm \ref{al:method}.

\subsection{Detail of Studied Methods} \label{app:studied method}
To show the compatibility of our method, we apply the DVR framework on four recommendation backbones, i.e., BRPMF~\cite{koren2009matrix}, NeuMF~\cite{he2017neural}, MGCF~\cite{wang2019neural}, and LightGCN~\cite{he2020lightgcn}. We select BPRMF due to its widespread adoption in recommendation systems and proven effectiveness in practical applications. NeuMF, an MLP-based approach, extends the capabilities of BPRMF by capturing intricate user-item relationships. We leverage GNN-based models, such as MGCF and LightGCN, known for their state-of-the-art performance and competitive outcomes across various techniques, to serve as the recommendation backbone. 

Based on these backbones, different versions of the DVR model are tailored to optimize diverse metrics. For simplicity, we designate models optimized for ranking accuracy as DVR-Loss, DVR-Recall, and DVR-NDCG. Likewise, models focused on diversity and fairness metrics are labeled as DVR-CC, DVR-ILD, and DVR-Gini.

We compare our framework with various data valuation methods for recommendations. BPR~\cite{10.5555/1795114.1795167} uniformly samples negative items and treats all training data equally in constructing the training objective. TCE-BPR and RCE-BPR are extensions of the TCE and RCE techniques \cite{10.1145/3437963.3441800}, aimed at dynamically filtering out noisy positive interactions during training based on loss values. In our implementation, we replace the original point-wise loss with a pair-wise ranking loss objective to ensure a fair comparison with these methods. AOBPR \cite{10.1145/2556195.2556248} enhances the BPR algorithm by incorporating adaptive sampling techniques that prioritize popular negative items. WBPR \cite{gantner2012personalized} assumes that unexplored popular items by a user are more likely to be true negatives. PRIS \cite{10.1145/3366423.3380187} assigns higher weights to informative negative samples using importance sampling. TIL-UI and TIL-MI \cite{wu2022adapting} learn the data value of training triplets through two aggregation strategies by optimizing the BPR loss within the training batch.

\subsection{Implementation Details} \label{app:implenmentation}
We optimize all models using the Adam optimizer with Xavier initialization \cite{glorot2010understanding} and maintain a fixed embedding size of 64 across all methods. When constructing the ranking loss objective, every positive item is associated with one sampled negative item for an efficient computation. Grid search is applied to choose learning rate and weight decay from $\left\{1e^{-4}, 1e^{-3}, 1e^{-2}, 1e^{-1}\right\}$ and $\left\{1e^{-6}, 1e^{-5}, 1e^{-4}, 1e^{-3}\right\}$. The backbone models NeuMF, MGCCF, and LightGCN utilize the provided implementations, with MGCF and LightGCN featuring two graph convolution layers. The total number of training epochs is set to 2000 for all models with an early stopping design. Given the initial training stages' limited information, we pre-train the recommendation model without data valuator for 1000 epochs to get meaningful embeddings. We set the number of the pre-training epochs to 1000. All experiments are conducted on GPU machines (NVIDIA GeForce RTX 3090).

\begin{algorithm}[H]
    \caption{The Proposed Method}
    \label{al:method}
    
    \textbf{Input:} Learning rates $\alpha$ and $\beta$, outer mini-batch size $B_1$, inner mini-batch size $B_2$, outer iteration count $T_1$, inner iteration count $T_2$, moving average window $W$, training pairs $\mathcal{D}_{1}=\{(u,i)\}_{k=1}^{L_1}$, validation pairs $\mathcal{D}_{2}=\{(u,i)\}_{k=1}^{L_2}$
    
    \textbf{Initialize:} parameters $\Theta$ and $\Lambda$, moving average $\delta=0$
    
    \begin{algorithmic}[1]
    \FOR{outer iteration $t_1=1,2,...,T_1$}
        \STATE Sample a mini-batch from the entire training dataset: $\mathcal{\hat{B}}=(u,i)_{k=1}^{B_1}\sim \mathcal{D}_1$
        \STATE Uniformly sample negative items $(j)_{k=1}^{B_1}$ for training pairs $(u,i)_{k=1}^{B_1}$ to get training data $\mathcal{B}=(u,i,j)_{k=1}^{B_1}$ for the recommendation model
        \FOR{$(u,i,j) \in \mathcal{B}$}
        \STATE Calculate the Shapley value by Eq. (\ref{eq:svcal}) and assign it to $w_{uij}$
        \ENDFOR
        \STATE Normalize the Shapley value $w_{uij}$ within the batch $\mathcal{B}$ as $\hat{w}_{uij}$ 
        \STATE Compute sample selection vector $s_{uij}=\text{Ber}(\hat{w}_{uij})$ from Bernoulli distribution
        \STATE Update the data valuator model by \ref{eq:mse}
        \FOR{inner iteration $t_2=1,2,...,T_2$}
        \STATE Sample a mini-batch $(u,i,j)_{m=1}^{B_2}\sim \mathcal{B}$
        \STATE Update the recommendation model:
    $$\Theta \leftarrow \Theta-\frac{\alpha}{B_2} \sum_{m=1}^{B_2} s_{uij} \cdot \nabla_\Theta \mathcal{L}_{\text{BPR}}(u,i,j;\Theta)$$
        \ENDFOR
    \STATE Update the data valuator:
    $$ \begin{array}{r}
    \Lambda \longleftarrow \Lambda - \beta [\mathcal{R}(\mathcal{D}_2, f(\Theta^*(\Lambda)))-\delta ]\\ \cdot \nabla_{\Lambda}log(\pi(\mathcal{B},(s_{uij})_{k=1}^{B_1};{\Lambda})
    \end{array}
    $$
    \STATE Update the moving average reward:
    $$
    \delta \leftarrow \frac{W-1}{W} \delta+\frac{1}{W} \mathcal{R}(\mathcal{D}_2, f(\Theta^*(\Lambda)))
    $$                               
    \ENDFOR
    \end{algorithmic}
\end{algorithm}
